# Supplementary material for: Deep(er) Reconstruction of Imaging Cherenkov Detectors with Swin Transformers and Normalizing Flow Models
Source: arXiv:2407.07376 source file (2024-07-10)
Supplement: Supplementary file 1 [file Appendix.tex]

%\newpage
\appendix

\section{Title Here} \label{app:complete}
